# Supplementary material for: Mitigating the source-side channel vulnerability by characterization of photon statistics
Source: arXiv:2308.14402 source file (2023-08-28)
Supplement: Supplementary file 1 [file appendix.tex]

\appendix

\section{Upper and lower limits of probability}
The weak coherent pulses follow poisonnian photon statistics and to characterise such a source its essential to give the rigourous bounds on $p_n$. Such bounds were formulated in \cite{Kumazawa:19} and the explicit formulas for the bounds calculated with $D=4$ are given below. Where, they defined $\tilde{c}_{\mathrm{obs}, r}:=c_{\mathrm{obs}, r} / c_{r, r}$, which reduces to $\tilde{c}_{\mathrm{obs}, r}=c_{\mathrm{obs}, r} /\left(r ! \eta^{r}\right)$ for the uniform cases of $\eta=\eta_{1}=\eta_{2}=\eta_{3}=\eta_{4}$. They are of $O(1)$ in the limit of $\eta \rightarrow 0$. To simplify the notations, they also defined $s_{j}:=\sum_{W \in I_{j}} \prod_{i \in W} \eta_{i} /\left(\begin{array}{c}D \\ j\end{array}\right)(j=2, \ldots, D)$, and $\xi_{i, j}:=s_{i} /\left(s_{j} \eta^{i-j}\right)-1(i, j=2, \ldots, D)$. The formula for the uniform case is simply given by setting $\xi_{i, j}=0$ for all $i, j$.

\begin{equation}
\begin{aligned}
&p_{0}^{L}=1-\tilde{c}_{\mathrm{obs}, 1}+\left[1-\left(1-3 \xi_{2,1}\right) \eta\right] \tilde{c}_{\mathrm{obs}, 2}\\
&-\left[1-\left(3-3 \xi_{3,2}\right) \eta+\left(2-12 \xi_{3,2}+6 \xi_{3,1}\right) \eta^{2}\right] \tilde{c}_{\mathrm{obs}, 3}\\
&+4\left(1+\xi_{4,3}\right) \eta\left[1-6 \eta+\left(11+3 \xi_{3,1}\right) \eta^{2}\right.\\
&\left.-6\left(1+\xi_{3,1}\right) \eta^{3}\right] \tilde{c}_{\mathrm{obs}, 4} \text {, }\\
\end{aligned}
\end{equation}

\begin{equation}
\begin{aligned}
&p_{0}^{U}=1-\tilde{c}_{\mathrm{obs}, 1}+\left[1-\left(1-3 \xi_{2,1}\right) \eta\right] \tilde{c}_{\mathrm{obs}, 2}\\
&-\left[1-\left(3-3 \xi_{3,2}\right) \eta+\left(2-12 \xi_{3,2}+6 \xi_{3,1}\right) \eta^{2}\right] \tilde{c}_{\text {obs, } 3}\\
&+\left[1-\left(6-2 \xi_{4,3}\right) \eta+\left(11+6 \xi_{2,1}-8 \xi_{3,2} / 3\right.\right.\\
&\left.-12 \xi_{4,3}+11 \xi_{4,2} / 3\right) \eta^{2}-\left(6+24 \xi_{2,1}-32 \xi_{3,2} / 3\right.\\
&\left.\left.-16 \xi_{4,3}+44 \xi_{4,2} / 3-6 \xi_{4,1}\right) \eta^{3}\right] \tilde{c}_{\text {obs }, 4} \text {, }\\
\end{aligned}
\end{equation}

\begin{equation}
\begin{aligned}
&p_{1}^{L}=\tilde{c}_{\mathrm{obs}, 1}-\left[2-\left(1-3 \xi_{2,1}\right) \eta\right] \tilde{c}_{\mathrm{obs}, 2}\\
&+\left[3-\left(6-6 \xi_{3,2}\right) \eta+\left(2-12 \xi_{3,2}+6 \xi_{3,1}\right) \eta^{2}\right] \tilde{c}_{\text {obs }, 3}\\
&-\left[4-\left(18-6 \xi_{4,3}\right) \eta+\left(22+12 \xi_{2,1}\right.\right.\\
&\left.-16 \xi_{3,2} / 3-24 \xi_{4,3}+22 \xi_{4,2} / 3\right) \eta^{2}\\
&-\left(6+24 \xi_{2,1}-32 \xi_{3,2} / 3\right.\\
&\left.\left.-16 \xi_{4,3}+44 \xi_{4,2} / 3-6 \xi_{4,1}\right) \eta^{3}\right] \tilde{c}_{\text {obs } 4,} \text {, }\\
\end{aligned}
\end{equation}

\begin{equation}
\begin{aligned}
&p_{1}^{U}=\tilde{c}_{\text {obs, } 1}-\left[2-\left(1-3 \xi_{2,1}\right) \eta\right] \tilde{c}_{\text {obs, } 2}\\
&+\left[3-\left(6-6 \xi_{3,2}\right) \eta+\left(2-12 \xi_{3,2}+6 \xi_{3,1}\right) \eta^{2}\right] \tilde{c}_{\text {obs, } 3}\\
&-4\left(1+\xi_{4,3}\right) \eta\left[3-12 \eta+\left(11+3 \xi_{3,1}\right) \eta^{2}\right] \tilde{c}_{\mathrm{obs}, 4} \text {, }\\
\end{aligned}
\end{equation}

\begin{equation}
\begin{aligned}
&p_{2}^{L}=\tilde{c}_{\mathrm{obs}, 2}-3\left[1-\left(1-\xi_{3,2}\right) \eta\right] \tilde{c}_{\mathrm{obs}, 3}\\
&+12\left(1+\xi_{4,3}\right) \eta(1-2 \eta) \tilde{c}_{\text {obs } 4,} \text {, }\\
\end{aligned}
\end{equation}

\begin{equation}
\begin{aligned}
&p_{2}^{U}=\tilde{c}_{\text {obs }, 2}-3\left[1-\left(1-\xi_{3,2}\right) \eta\right] \tilde{c}_{\text {obs }, 3}\\
&+\left[6-\left(18-6 \xi_{4,3}\right) \eta+\left(11+6 \xi_{2,1}\right.\right.\\
&\left.\left.-8 \xi_{3,2} / 3-12 \xi_{4,3}+11 \xi_{4,2} / 3\right) \eta^{2}\right] \tilde{c}_{\text {obs }, 4},\\
\end{aligned}
\end{equation}

\begin{equation}
\begin{aligned}
&p_{3}^{L}=\tilde{c}_{\mathrm{obs}, 3}-\left[4-2\left(3-\xi_{4,3}\right) \eta\right] \tilde{c}_{\mathrm{obs}, 4},\\
\end{aligned}
\end{equation}

\begin{equation}
\begin{aligned}
&p_{3}^{U}=\tilde{c}_{\text {obs }, 3}-4\left(1+\xi_{4,3}\right) \eta \tilde{c}_{\text {obs }, 4} \text {, }\\
\end{aligned}
\end{equation}

\begin{equation}
\begin{aligned}
&p_{\geq 4}^{L}=4 !\left(1+\xi_{4,1}\right) \eta^{4} \tilde{c}_{\text {obs }, 4},\\
\end{aligned}
\end{equation}

\begin{equation}
\begin{aligned}
&p_{\geq 4}^{U}=\tilde{c}_{\text {obs } 4 .} \text {. }
\end{aligned}
\end{equation}
